# Supplementary material for: From Mott to not: phenomenology of overdoped cuprates
Source: arXiv:1902.08286 ancillary file (2019-02-21)
Supplement: Supplementary file 1 [file overdopedSM.pdf]

# From Mott to not: phenomenology of overdoped cuprates

## SUPPLEMENTAL MATERIAL

N. R. Lee-Hone, H. U. Özdemir, V. Mishra, D. M. Broun, P. J. Hirschfeld

### Fermi surface averages

To properly capture the phenomenology of the overdoped cuprates it is essential to begin with realistic models of the energy dispersion and Fermi surface, as discussed in Ref. 23. The Fermi surface average is then defined as

$$\langle ... \rangle_{\rm FS} \equiv \frac{1}{N_0} \int_0^{2\pi} N_\phi(...) d\phi, \tag{S1}$$

where the angle-dependent density of states is

$$N_\phi = \frac{1}{2\pi^2 \hbar d} \frac{|k_F|^2}{\mathbf{k}_F \cdot \mathbf{v}_F}. \tag{S2}$$

Here $N_0$ is the total density of states and $d$ is the average spacing between the copper-oxide layers: $d = 13.15/2 = 6.57$ Å for LSCO; $d = 23.2/2 = 11.6$ Å for Tl-2201. The angle-dependent Fermi momentum, $\mathbf{k}_F$, and Fermi velocity, $\mathbf{v}_F$ are obtained from tight-binding parameterizations of ARPES-derived energy dispersions.

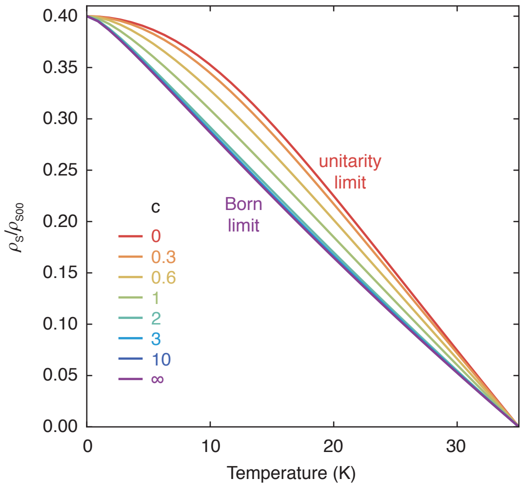


FIG. S1. Superfluid density calculated using the band structure of LSCO and a $d$-wave order parameter, for various impurity phase shifts. In each case the underlying scattering parameter $\Gamma_N$ has been adjusted to fix the zero-temperature superfluid fraction at $\rho_s/\rho_{s00} = 0.4$, corresponding to the level of pair breaking in near optimally doped LSCO [23, 32]. Note that the Born limit results are nearly indistinguishable from those of the full $t$-matrix evaluation up to a phase shift parameter of $c \simeq 2$. This illustrates the broad generality of the Born limit, which in practice extends over a wide regime of scatterer densities and scattering strengths. Details of the superfluid density calculation are given in Ref. 23.

### ARPES-derived dispersions for LSCO and Tl-2201

For LSCO, tight-binding parameterizations of the doping-dependent Fermi surface were obtained from a series of ARPES measurements at different dopings [45]. These were the basis of our earlier calculations in Refs. 23 and 24, and were essential to providing an accurate account of the electrodynamic response in LSCO, in particular the nearly linear temperature dependence of superfluid density between $T = 0$ and $T_c$ shown in Fig. S1, which is not obtained in the case of an isotropic Fermi surface. We note that the ARPES tight-binding fits in LSCO were carried out over the full bandwidth and do not capture the effects of many-body renormalization close to the Fermi level, as pointed out by the authors of Ref. 45. As a result, the conductivity calculations in Ref. 24 required an overall renormalization of plasma frequency by a factor of 0.3, consistent with previous work on LSCO [25].

For overdoped Tl-2201, Plate et al., [46] carried out a tight-binding fit to low energy ARPES spectra on $T_c = 30$ K material and obtained the following dispersion:

$$\begin{aligned}\epsilon_{\mathbf{k}} &= \mu + \frac{t_1}{2}\left(\cos k_x + \cos k_y\right) + t_2 \cos k_x \cos k_y \\ &+ \frac{t_3}{2}\left(\cos 2k_x + \cos 2k_y\right) + \frac{t_4}{2}\left(\cos 2k_x \cos k_y + \cos k_x \cos 2k_y\right) \\ &+ t_5 \cos 2k_x \cos 2k_y \ ,\end{aligned} \tag{S3}$$

in which wave-vector $\mathbf{k} = (k_x, k_y)$ is measured in units of inverse lattice parameter, with hopping parameters $t_1 = -0.725$, $t_2 = 0.302$, $t_3 = 0.0159$, $t_4 = -0.0805$ and $t_5 = 0.0034$ eV. In the absence of ARPES spectra at other dopings, we model the doping dependence of the dispersion by a rigid band shift, a relatively safe assumption as Tl-2201 is situated far from a van Hove crossing. In contrast to LSCO, we note that the ARPES tight-binding fits for Tl-2201 were carried out at very low energies (10s of meV) and fully capture the many-body flattening of the dispersion near the Fermi level. As a result, no additional renormalization factors are required. In particular, the Tl-2201 superfluid density plotted in Fig. 1(b) and the thermal conductivity plotted in Fig. 3 are fully dimensionful quantities calculated directly from the tight-binding dispersion (Eq. S3), with no adjustable band parameters.

### The Born limit and impurity phase shift

Most of the analysis presented here, in addition to the results in Refs. 23 and 24, was obtained assuming weak scatterers in the Born limit, plus a small admixture of strong scatterers. However, the argument that the dopant atoms located out of the $CuO_2$ plane correspond to such an extremely weak scattering potential should be examined critically, par-

ticularly in the case of LSCO where the Sr dopants are located only about 2 Å above the plane. In Fig. S1 we show that in terms of the dimensionless parameter $c = 2/(\pi V_{\rm imp} N_0)$, where $V_{\rm imp}$ is the impurity potential and $N_0$ is the total density of states at the Fermi level, there is in fact a wide range of weak to intermediate-strength scattering potentials that produce results virtually identical to the Born limit, illustrating that the Born limit is in fact a regime of broad physical applicability. Since $N_0$ in our ARPES-derived band structures is respectively 7.5 eV$^{-1}$ and 3.5 eV$^{-1}$ (per formula unit) for LSCO and Tl-2201, this means that impurities with potentials up to $\sim$ 0.1 eV (formula unit) are compatible with the Born limit results presented here. An upper bound on the Sr scattering strength can be obtained by attributing all scattering to the Sr dopants and relating this to the normal-state elastic scattering rate $\Gamma_N$. Assuming that the scatterers are indeed close to the Born limit, $\Gamma_N = \frac{\pi}{2} n_i N_0 V_{\rm imp}^2$. For overdoped LSCO, we set the Sr impurity concentration at $n_i = 0.2$ per formula unit and, as above, a total density of states $N_0 = 7.5$ eV$^{-1}$.With our current choice $\Gamma_N = 18\pi$ K, confirmed qualitatively by analysis of optical data in Ref. 24, we obtain $V_{\rm imp} \approx 45$ meV. This establishes that the Sr dopants are indeed in the weak scattering regime. We note that this is a worst case estimate of the Sr scattering strength, in particular because it ignores the presence of oxygen vacancies.

### Entropy conserving analysis of residual heat capacity in Tl-2201

The best data on the doping dependent specific heat of Tl-2201 come from the study on polycrystalline material by Loram et al., reported in Ref. 42. While the differential calorimetry method works very well at high temperatures, successfully isolating the electronic specific heat from a large phonon background, clear Schottky contributions are visible at low temperature and are more difficult to subtract. To estimate the residual value of the Sommerfeld coefficient, $\gamma = C(T)/T$, we have fit to $\gamma(T)$ in such a way that the change in entropy,

$$\Delta S = \int_0^{T_N} \gamma(T)\, dT \ , \qquad \text{(S4)}$$

between $T = 0$ and some $T_N > T_c$ is the same in the superconductor and normal states. These equal area constructions are plotted in Fig. S2 for the three highest dopings (three lowest $T_c$'s) and allow a more reliable extrapolation beneath the Schottky contributions.

### Quasiparticle Doppler shift and vortex state in the semiclassical approximation

A Bogoliubov quasiparticle with Fermi velocity $\mathbf{v_k}$, in a uniform superflow characterized by gauge-invariant pair momentum $\mathbf{p}_s = \hbar\mathbf{Q}$, experiences a Doppler shift $\frac{1}{2}\mathbf{p}_s \cdot \mathbf{v_k}$. In the semiclassical approximation, it is assumed that the dominant

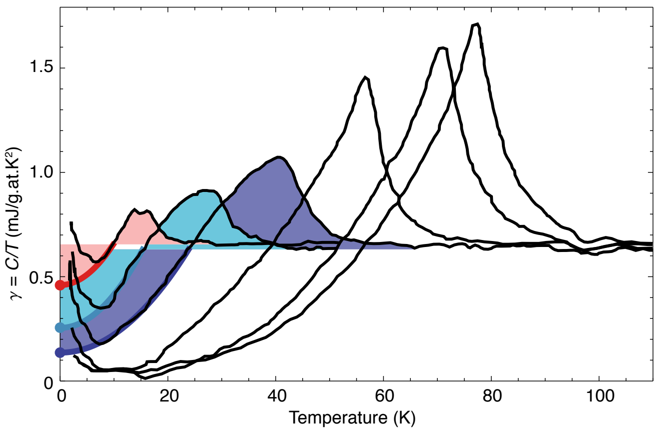


FIG. S2. Heat capacity data for overdoped Tl-2201 from Loram et al., Ref. 42, showing the entropy-conserving fits used to estimate the residual Sommerfeld coefficient at the three highest dopings (three lowest $T_c$'s).

effect of magnetic field in the vortex state is via the Doppler shift of the quasiparticle energies by the *local* superflow field. This is believed to be particularly important in $d$-wave superconductors, in which the nodal gap results in a significant density of delocalized excitations outside the vortex cores, and is associated with the appearance of $\sqrt{H}$ behaviour in the clean limit [48, 49, 57]. To represent the vortex lattice, we follow Ref. 50 and use an approach that applies in the field regime $H_{c1} \ll H \ll H_{c2}$, where Meissner screening can be ignored. For magnetic field applied along the $\hat{\mathbf{z}}$ direction, the superflow field at position $\mathbf{r}$ takes the form

$$\mathbf{Q}(\mathbf{r}) = (Q_x, Q_y) = \sum_i \frac{\hat{\mathbf{z}} \times (\mathbf{r} - \mathbf{r}_i)}{(\mathbf{r} - \mathbf{r}_i)^2} \ , \qquad \text{(S5)}$$

where $\mathbf{r}_i$ is the center of the $i^{\rm th}$ vortex. We are specifically interested in the cases of square and triangular (hexagonal) vortex lattices, as both are relevant to the cuprates. As in Ref. 50, we use a Fourier method to first carry out the sum over a single row of vortices. For a line of vortices centered on the origin and spaced by distance $a$ along the $x$ axis, we find the $x$ and $y$ components of the flow field to be, respectively:

$$Q_{1x}(x,y) = \frac{\pi}{a} \frac{\sinh\left(\frac{2\pi y}{a}\right)}{\cos\left(\frac{2\pi x}{a}\right) - \cosh\left(\frac{2\pi y}{a}\right)} \ , \qquad \text{(S6)}$$

$$Q_{1y}(x,y) = -\frac{\pi}{a} \frac{\sin\left(\frac{2\pi x}{a}\right)}{\cos\left(\frac{2\pi x}{a}\right) - \cosh\left(\frac{2\pi y}{a}\right)} \ . \qquad \text{(S7)}$$

To obtain the flow field for the full vortex lattice, the sum over rows is carried out numerically and converges sufficiently rapidly that only a few rows in the vicinity of the point of interest need be included. In particular, the $1/r$ divergence at the origin is captured exactly by the zeroth row. For the square

vortex lattice, the final result is

$$Q_x(x,y) = \frac{2\pi y}{a^2} + \sum_n Q_{1x}(x, y-na) \tag{S8}$$

$$= \frac{2\pi y}{a^2} + \frac{\pi}{a}\sum_n \frac{\sinh\left(\frac{2\pi y}{a} - 2\pi n\right)}{\cos\left(\frac{2\pi x}{a}\right) - \cosh\left(\frac{2\pi y}{a} - 2\pi n\right)}\,, \tag{S9}$$

$$Q_y(x,y) = \sum_n Q_{1y}(x, y-na) \tag{S10}$$

$$= -\frac{\pi}{a}\sum_n \frac{\sin\left(\frac{2\pi x}{a}\right)}{\cos\left(\frac{2\pi x}{a}\right) - \cosh\left(\frac{2\pi y}{a} - 2\pi n\right)}\,, \tag{S11}$$

where $n$ is a set of integers and the linear term in $Q_x$ is a correction arising from the long-range nature of $Q_{1x}$. For the triangular (hexagonal) vortex lattice

$$Q_x(x,y) = \frac{4\pi y}{\sqrt{3}a^2} + \sum_n Q_{1x}\left(x - na/2, y - \sqrt{3}na/2\right) \tag{S12}$$

$$= \frac{4\pi y}{\sqrt{3}a^2} + \frac{\pi}{a}\sum_n \frac{\sinh\left(\frac{2\pi y}{a} - \sqrt{3}n\pi\right)}{\cos\left(\frac{2\pi x}{a} - n\pi\right) - \cosh\left(\frac{2\pi y}{a} - \sqrt{3}n\pi\right)}\,, \tag{S13}$$

$$Q_y(x,y) = \sum_n Q_{1y}\left(x - na/2, y - \sqrt{3}na/2\right) \tag{S14}$$

$$= -\frac{\pi}{a}\sum_n \frac{\sin\left(\frac{2\pi x}{a} - n\pi\right)}{\cos\left(\frac{2\pi x}{a} - n\pi\right) - \cosh\left(\frac{2\pi y}{a} - \sqrt{3}n\pi\right)}\,. \tag{S15}$$

The small-angle neutron scattering experiments in Ref. 43 show that the vortex lattice in overdoped LSCO adopts a square structure above a field of 0.4 T, with primitive vectors aligned along the Cu-O bond directions. Such a square lattice has therefore been used in the calculations of field-dependent specific heat shown in Fig. 2(c). The results for a triangular (hexagonal) vortex lattice are qualitatively similar but approximately 3-5% larger.

To take into account order parameter suppression near the vortex core, we employ the Clem model [58], in which the normalized order parameter takes the form

$$\frac{\Delta(\rho)}{\Delta_\infty} = \frac{\rho}{(\rho^2 + \xi_v^2)^{1/2}}\,. \tag{S16}$$

Here $\Delta_\infty$ is the gap magnitude in the uniform limit, obtained from solution of the gap equation, Eq. 3, in zero field, and $\rho$ is the radial displacement from the vortex center. In strongly type-II materials, the variational core radius parameter $\xi_v \to \sqrt{2}\xi$ [58], allowing its value to be set from magnetoresistive measurements of upper critical field in LSCO [59].

Spatial averages over the vortex-lattice unit cell are carried out by Monte-Carlo integration, using a total of 50,000 samples for each field point, based on pseudorandom Halton sequences generated from randomly chosen coprime pairs. The Halton sequences provide more uniform sampling and faster convergence than purely random Monte Carlo. At each sampling point in the vortex-lattice unit cell, a full Fermi-surface integral is then carried out, rather than the usual nodal approximation, in order to accurately evaluate the density of states in the *local* superflow.

In Fig. 2(c), it is interesting that the coefficient $A$ of a $C(T \to 0, H)/T = A\sqrt{H}$ term fit to the Wang et al. [41] data on overdoped LSCO gives a nonmonotonic variation of $A$ with $x$, as does the theory. This can be possibly understood as an initial increase of the vortex core size as $\Delta$ decreases, together with a subsequent suppression of $A$ due to disorder. However the agreement in the figure is only qualitative, not quantitative. While we have gone to some lengths to perform the most accurate semiclassical calculations appropriate to the systems studied, there is some reason to doubt that quantitative results including weak disorder can be obtained in this limit. The Volovik effect is a zero-temperature property valid for $H_{c1} \ll H \ll H_{c2}$. At low temperatures and energies, the mean free path of a quasiparticle experiencing Born scattering may become very long, larger than the intervortex spacing, such that the implicit assumption of a local self energy in Eq. 6 is no longer appropriate. Furthermore, we are extending the theory to significant fractions of $H_{c2}$ for the more overdoped cases. A more complete treatment at high fields along the lines of the Brandt-Pesch-Tewordt theory [60] may be required to describe these data accurately.
